# Supplementary material for: Mechanism to Generate a Two-Dimensional Electron Gas at the Surface of the Charge-Ordered Semiconductor BaBiO3
Source: arXiv:1209.4271 source file (2013-05-21)
Supplement: Supplementary file 1 [file def_babio3-supp.tex]

\def\babio3{BaBiO$_3$}
\def\bakbio3{Ba$_{1-x}$K$_x$BiO$_3$}
\def\bapbio3{BaPb$_{1-y}$Bi$_y$O$_3$}

\def\bi3{Bi$^{3+}$}
\def\bi4{Bi$^{4+}$}
\def\bi5{Bi$^{5+}$}
